# Supplementary material for: Gapped Excitations of unconventional FQHE states in the Second Landau Level
Source: arXiv:1507.04939 source file (2015-10-05)
Supplement: Supplementary file 1 [file Supplemental_Material_Wurstbauer_et_al.pdf]

Supplemental Material

# Gapped Excitations of unconventional FQHE states in the Second Landau Level

U. Wurstbauer[1,2], A. L. Levy[3], A. Pinczuk[3,4], K. W. West[5], L. N. Pfeiffer[5], M. J. Manfra[6,7,8], G. Gardner[7], J. Watson[6]

[1]*Walter Schottky Institut and Physik-Department, Technische Universität München, 85748 Garching, Germany*
[2]*Nanosystems Initiative Munich (NIM), Schellingstr. 4, 80799 München, Germany*
[3]*Department of Physics, Columbia University, New York, NY 10027, USA*
[4]*Department of Applied Physics and Applied Mathematics, Columbia University, NY, New York 10027, USA*
[5]*Department of Electrical Engineering, Princeton University, Princeton, NJ 08544, USA*
[6]*Department of Physics and Astronomy, Birck Nanotechnology Center, Purdue University, West Lafayette, IN, USA*
[7]*School of Materials Engineering, Birck Nanotechnology Center, Purdue University, West Lafayette, IN, USA*
[8]*School of Electrical and Computer Engineering Birck Nanotechnology Center Purdue University, West Lafayette, IN, USA*

## 1) Resonant enhancement of inelastic light scattering

Inelastic light scattering by collective excitations of fluids of the FQHE can only be observed under optimized resonance conditions [1]. Resonant enhancements are due to intermediate interband optical transitions involving conduction and valence subbands of the GaAs quantum well that is host to the electron fluids. In a strong magnetic field the complex structure of valence Landau levels (LL's) modifies

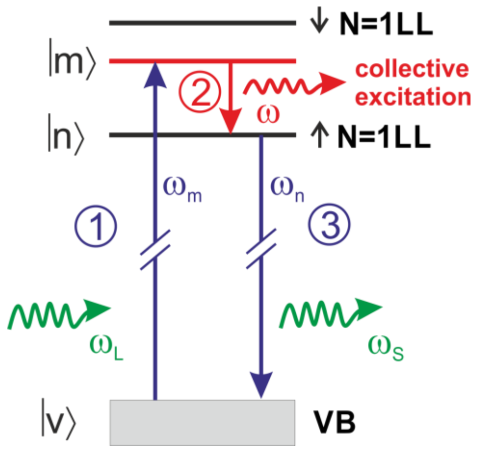


**Figure S1**: Schematic transition diagram for three step RILS processes for a collective excitation at energy $\omega$. The circled numbers indicate the time-order of the transitions. The energies $\omega_m$ and $\omega_n$ are across the fundamental optical band gap of GaAs quantum wells.

the optical matrix elements [2]. These changes of the optical matrix elements have major impact on polarization selection rules in resonant inelastic light scattering (RILS) in a magnetic field.

RILS by collective excitations can be described within 3rd order time-dependent perturbation theory. The three virtual transitions are sketched in Fig. S1. In the first step an incoming photon of energy $\omega_L$ is annihilated and an electron from a valence subband state (vb) is promoted to an intermediate state $|m\rangle$ in a conduction subband (cb). The state $|m\rangle$ is in the N=1 electron Landau level (LL), and the hole $|v\rangle$ is in a state of a valence LL. In the second step electron-electron interactions $H_{ee}$ cause a transition from $|m\rangle$ to the second intermediate state $|n\rangle$, also in the N=1 LL, with creation of a collective quasiparticle excitation of the electron fluid. In the third and last step there is the recombination of $|n\rangle$ and $|v\rangle$ with emission of the scattered photon of energy $\omega_S$. The energy of the quasiparticle excitation in is $\omega = \omega_L - \omega_S$.

For the three step process described in Fig. S1 the scattering intensity can be written as [3]:

$$I(\omega) \propto \left| \sum_{m,n} \frac{\langle v|H'_{\text{int}}|n\rangle\langle n|H_{ee}|m\rangle\langle m|H'_{\text{int}}|v\rangle}{(\omega_s - \omega_n)(\omega_L - \omega_m)} \right|^2 \tag{1}$$

In expression (1) $\omega_{m(n)}$ is the energy of the vertical transition $|v\rangle \rightarrow |m\rangle$ ($|n\rangle \rightarrow |v\rangle$). The light scattering intensity reaches its maximum at resonance, when a denominator in Eq. (1) is vanishingly small.

## 2) Sample and experimental set-up

GaAs samples containing the heterostructures with a length of about 20 mm and a width of 5mm are mounted on the cold finger of a $^3He/^4He$ dilution refrigerator equipped with 16 T superconducting magnet and bottom windows for direct optical access. The RILS and resonant Rayleigh scattering (RRS) spectra are excited with linearly polarized light by a tunable Ti:Sapphire laser at an incident power below $10^{-4}$ W/ cm$^2$. The energy of the exciting light $\omega_L$ is tuned to be close to the optical emission from the N = 1 LL to achieve resonant enhancement. The used backscattering geometry is sketched in inset of Fig. 1(a) in the main manuscript. The sample is tilted at an angle $\theta$ = 20°or $\theta$ = 25° respectively. The tilt angle results in a small in-plane magnetic field component $B_{//}$.

The polarization of incoming and scattered light is denoted with V and H as sketched in inset of Fig. 1(a) of the main manuscript. The scattered light is analyzed with a triple grating spectrometer. The gratings simultaneously serve as analyzer and consequently the polarization of the recorded scattered light is always *V*. The incoming light is *H* or *V* polarized resulting in a light scattering geometry that is either cross-polarized *(H,V)* or co-polarized (*V,V*). *V* polarized light has a small component parallel to $B_{//}$ and *H* polarized light is perpendicular to $B_{//}$ as shown in inset to Fig 1(a) of the of the main manuscript.

## 3) Identification of the filling factor

*(a) From resonant inelastic light scattering of spin waves near filling factor ν=3*

For states in the second LL (N=1) the magnetic field for filling factor ν=3 can be determined directly by RILS measurements of the long wavelength spin wave (SW) mode of this fully spin polarized state. The mode is at $E_Z$, the bare Zeeman energy of GaAs. From this determination, the magnetic fields for any filling in the N=1 LL are readily calculated.

Figure S2 describes the procedure by displaying resonance enhancement of RILS measurements of the SW mode at filling factor ν=3±0.2 taken in (H,V) polarization geometry. It is worth mentioning that the very sharp SW mode at ν=3 is observable only under extreme resonance conditions (close to the N=1L spin up emission). The very intense RILS SW mode completely disappears by changing the incoming photon energy

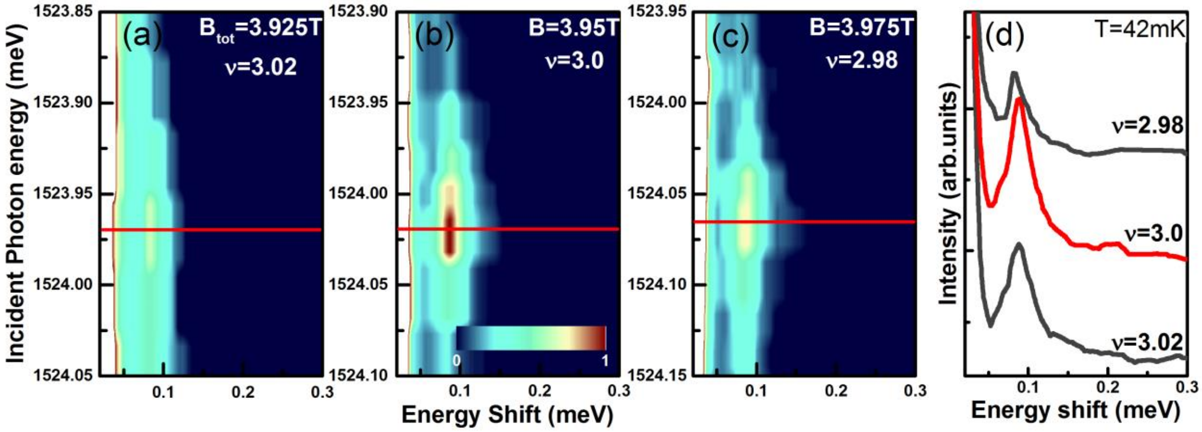


**Figure S2:** Color plot of the RILS intensities at filling factor ν=3.02 (a), ν=3.0 (b) and ν=2.98 (c) as a function of incident photon energy. Resonant enhancement of spin wave mode at the bare $E_Z$ is achieved only under extreme resonant conditions in a very narrow range of photon energies. The SW intensity is significantly reduced for small changes in filling factor away from ν=3. (d) Comparison of the resonantly enhanced spin wave modes from spectra shown in (a-c) (marked by the red line). The spin wave signal is significantly reduced for small deviations in filling factor of δν=±0.2 away from ν=3. All spectra are taken at a temperature of T = 42mK and in (H,V)-polarization geometry.

by only $\delta\omega_L$ =60μeV. It is clearly apparent that minor changes of the filling factor significantly lower the intensity of the SW peak at $E_Z$. A little change in filling factor of only δν=±0.02 from ν=3 to ν=2.98 and ν=3.02 significantly reduces the SW mode intensity clearly displaying filling factor 3. This reduction is caused by lowering of spin polarization with changes in filling factor near ν=3. With this procedure the magnetic field for ν=3 can be determined very precisely from the SW mode intensity in RILS measurements. Therefore, the accurate filling factor can be identified as a function of magnetic field in the N=1 LL. From these measurements, the two-dimensional electron density of the investigated sample yields n=2.6 $10^{11}$ $cm^{-2}$.

*(b) From emission measurements around filling factor ν=3*

An alternative measurement is the determination of the filling factor ν=3 from photoluminescence measurements. The emission from recombination of an electron residing in the N=1LL spin up branch with a photo-excited valence hole has a maximum exactly at filling factor ν=3. As shown in figure S3(a), the emission intensity from the N=1LL is largest at $B_{tot}$= 3.95T and is already reduced for changes in the magnetic field by ±25mT. This behavior identifies that ν=3 is at $B_{tot}$= 3.95T in excellent agreement with the SW investigations shown in figure S2. We would like to point out that both methods to determine the filling factor namely RILS by spin-wave and photoluminescence spectroscopy with emphasis to the N=1LL emission are quite accurate and reliable. Since disorder is a larger impact in photoluminescence than RILS spectroscopy, RILS measurements of spin-wave modes is the most reliable method to optically determine the filling factor with a very high precision without the need of contacts.

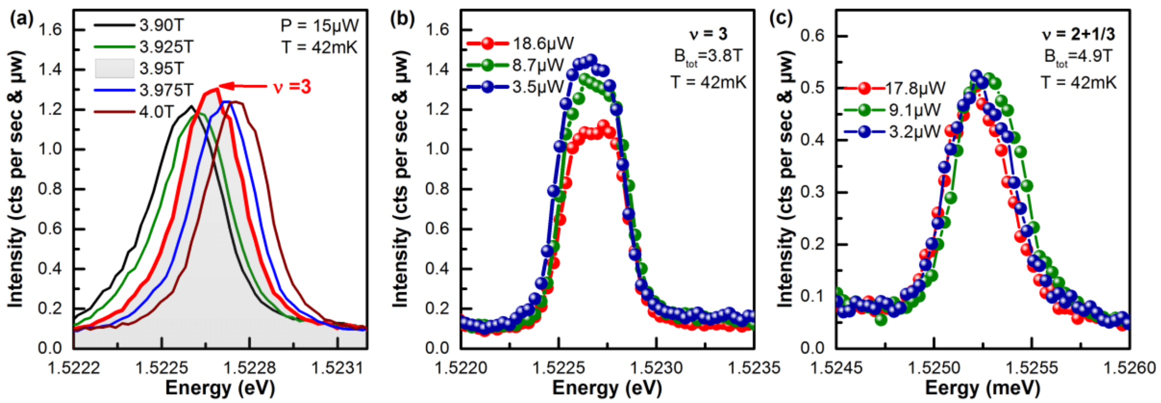


**Figure S3:** (a) Emission from the N=1 spin-up Landau level for different values of the total magnetic field $B_{tot}$. Filling factor ν=3 is determined from the most magnetic field, where the emission is most intense. (b) Power dependent emission of photo-excited e-h pairs at filling factor ν=3 (b) and ν=2+1/3 (c).

## 4) Stability of two-dimensional electron density under light irradiation

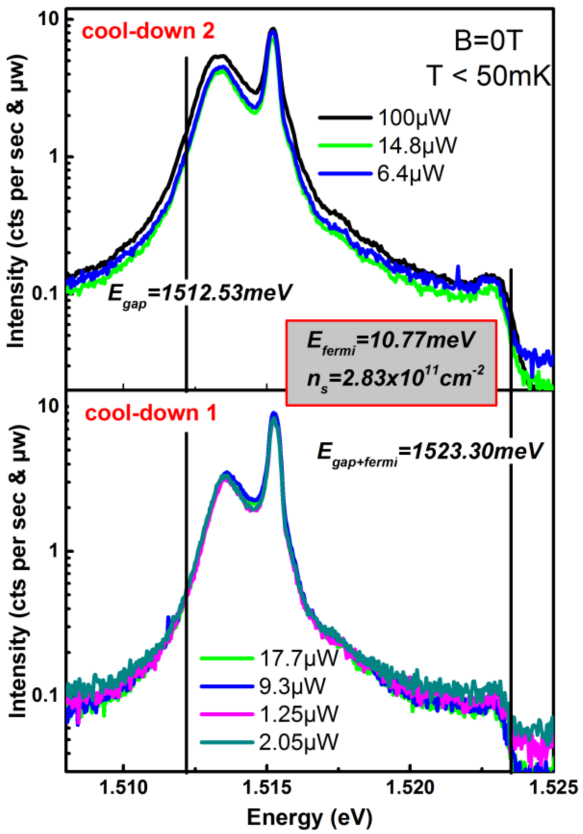


**Figure S4:** Photoluminescence intensities for different light intensities at B = 0T and T = 42mK ranging over two orders of magnitude. The density is determined directly after the neutral density filters and is subject to reduction by a fixed factor at the sample surface due to losses on optical elements and set of windows through the cryostat. The density refers to the density of a macroscopically large spherical spot with a constant length of a few mm and a width larger than 300μm. Data from different cool-downs are shown.

The immunity of the 2D charge carrier density against varying illumination intensity and/or application of a magnetic field is unambiguously required for reliable optical studies in the FQHE regime, particularly the weak states in the SLL. Here, the heterostructures were special designed and optimized for optical experiments and the stability of the charger carrier density was investigated at 4K and also at 42mK without and with an applied magnetic field. Power-dependent photoluminescence spectra at 42mK and B=0T are plotted in figure S4 for the first cool-down (lower panel) and a second cool-down (upper panel). Both, low energy onset at $E_{gap}$=1512.53meV defining the band-edge as well as the large energy cut-off at $E_{gap} + E_{fermi}$ = 1523.30meV of marking the Fermi edge do not show any modification with changing the light intensity over almost two orders of magnitude. The sample show nearly the same emission spectra at both cool-down highlighting the extraordinary stability and quality of the heterostructure. The Fermi energy $E_{fermi}$ and consequently the 2D charge carrier density can be determined from the energy difference between $E_{gap}$ and $E_{gap}$+$E_{fermi}$ and constitute $n_s = 2.83\times10^{11}$ cm$^{-2}$. This value is in good agreement

with the determination of filling factor ν=3 from RILS and PL measurements at $B_{tot}$=3.95T corresponding to $B_{\perp}$= 2.58T at a tilt angle of θ≈25° for cool-down 2. Cool-down 1 was performed at a tilt angle of θ≈20° and consistently filling factor ν=3 was determined to be at $B_{tot}$= 3.80T in RILS measurements. There are some uncertainties in determination of the exact tilt angle and also in the determination of the charge carrier density from B=0T photoluminescence measurements. For this reason, the filling factor was for each cool-down identified by RILS measurement of the SW mode presented in 2(a), a way to purely optically determine the filling factor with an outstanding precision.

We further verified the stability and power independency of the charge carrier density in presence of an applied magnetic field. In figure S3 are power dependent emission spectra from the N=1LL exemplarily shown for filling factor ν=3 (figure S3(b)) and for filling factor ν=2+1/3 (figure S3(c)). It is evident that the position of the emission spectra and hence the charge carrier density is absolutely stable in presence of an applied magnetic field and for various excitation intensities.

## 5) Temperature dependent RILS measurements at ν=2+1/3

Figure S5 displays the temperature dependency of the evolution of the lowest energy modes with excitation energy in RILS spectra for filling factor ν=2+1/3. The RILS intensity of the band of modes labeled $E_g$ is interpreted as gapped lowest energy neutral excitations of the 2+1/3 FQHE state. The mode intensities of the $E_g$ band are already significantly reduced by raising the temperature from 42mK to 100mK, are greatly reduced for 250mK and the modes are absent by raising the temperature to 600mK. Similarly, the mode at $E_{DOS}$ gets broadened and is greatly reduced in intensity by increasing the temperature to 600mK. The observed temperature dependency together with the filling factor

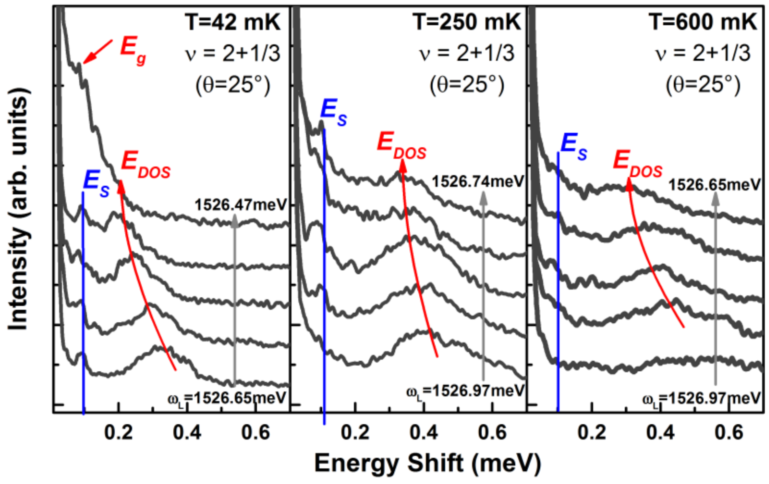


**Figure S5:** Temperature dependent RILS spectra at ν = 2+1/3 for T = 42mK, 250mK and 600mK measured in (H,V) geometry, θ=25°. The lowest energy band of modes $E_g$ is already absent at 250mK. The dispersive mode $E_{DOS}$ is significantly weakened and broadened by increasing the temperature. The mode $E_S$ is slightly weakened and broadened for the highest temperature at 600mK.

dependence corroborated the interpretation of the modes as collective lowest energy neutral excitations of the incompressible FQHE state at $\nu$ = 2+1/3.

The mode at $E_s$ interpreted as pure spin-mode exhibits a less significant temperature dependence. The mode gets broadened with increasing temperature, but the integrated intensity is less affected by raising the temperature compared to the charge modes. This finding is in agreement with the interpretation of spin wave mode indicating a large amount of spin-polarization. A loss of spin polarization by thermal activation of individual spin flips is in agreement with the observed temperature dependence of the $E_s$ mode as shown in figure S5.

## 6) Magnetic field dependent RILS measurements around ν=2+1/3

Figure S6 summarizes the magnetic field dependence of the RILS mode around filling factor $\nu$= 2+1/3. Even very small changes in the total magnetic field of $\Delta B_T \approx \pm 5$mT leading to a variation in filling factor as little as $\Delta\nu \approx 0.03$ cause a distinct reduction and broadening or even the disappearance of the RILS modes of the 2+1/3 state similar as reported in the main manuscript for the 2+2/5 and 2+3/8 states. The mode(s) labeled $E_g$ and interpreted at the lowest energy charge mode of the incompressible quantum fluid at 2+1/3 are most sensitive to the variation in filling factor, whereas the mode $E_S$ interpreted as spin wave mode is less sensitive to variation in filling factor as expected from the interpretation. Overall the filling factor

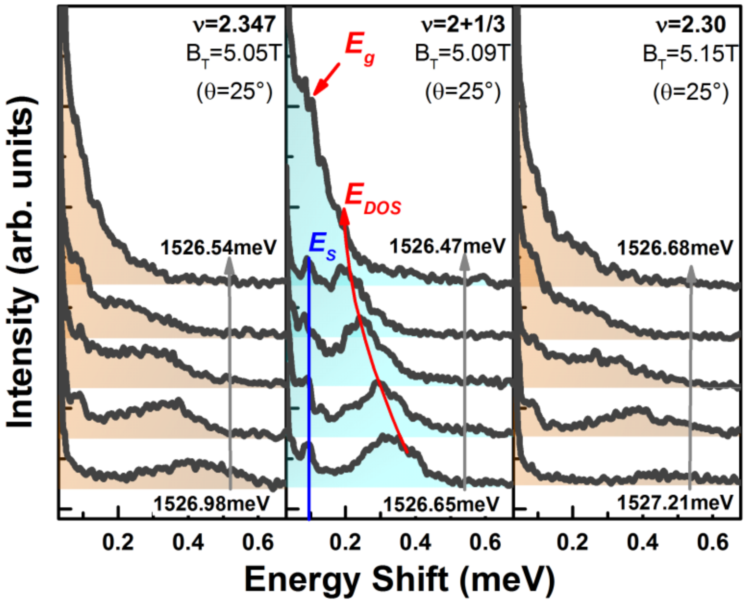


**Figure S6**: Filling factor dependence of RILS spectra around $\nu$ = 2+1/3. The spectra are shifted vertically for clarity. All observed, resonantly enhanced modes exhibit a striking filling factor dependence and are only well developed for $\nu$=2+1/3. Small changes in the filling factor of only $\Delta\nu$=0.03 significantly alters the RILS spectra and the well-developed modes are drastically weakened and broadened and can hardly be identified. All spectra are taken at a temperature of T = 42mK, in (H,V)-polarization geometry and a tilt angle $\theta$ = 25°.

supports the interpretation that the RILS modes can be interpreted as the lowest energy modes of the FQHE state at 2+1/3.

## 7) Polarization dependent Resonant Rayleigh scattering measurements around ν=2+2/5

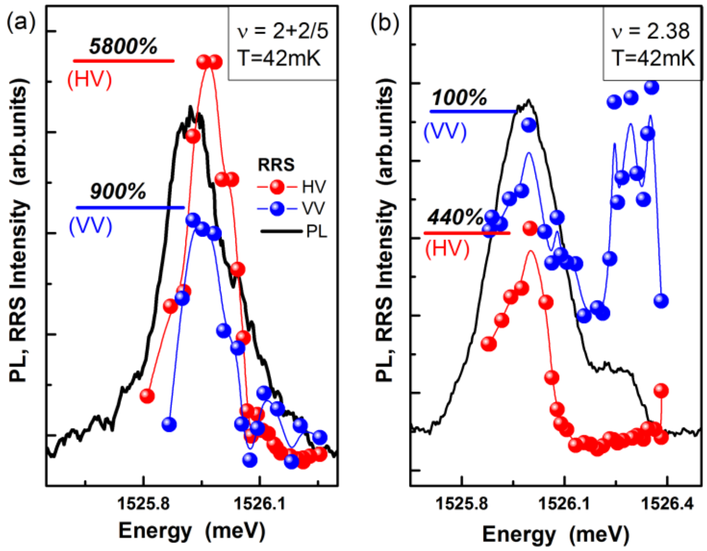


**Figure S6:** Photoluminescence spectra (black trace) and RRS data in co-polarized geometry (V,V) (blue dots) and cross-polarized geometry (H,V) *(red dots)* from the N=1 spin up Landau Level at ν=2+2/5=2.4 (a) and ν=2.38 (b). The solid lines in the RRS spectra are guides to the eyes. The resonant conditions in RRS overlap the emission peak in the PL spectra. (a) At ν=2+2/5, the peak of the RRS signal constitute an enhancement of 5800% and 900% in (H,V) and (V,V) geometry, respectively. (b) At ν=2.38, the RRS signal is enhanced by 440% and 100% in (H,V) and (V,V) geometry, respectively. The enhancement is generally stronger in (H,V) geometry. The RRS signal is drastically reduced by changing the filling factor of only δν=0.02 away from+2/5 to ν=2.38.

In Figure S6, emission spectra and Resonant Rayleigh scattering (RRS) spectra taken in (H,V) and (V,V) geometry from the N=1 LL (spin up branch) taken at filling factors ν=2+2/5 and ν=2.38 at base temperature (T = 42mK) are displayed. *H* and *V* denotes the linear polarization of the incoming and scattered light, respectively. The direction of the light polarization is such that *H*-direction is oriented perpendicular to the in-plane component of the magnetic field $B_{//}$ and *V*-direction has in the QW plane a small component parallel to $B_{//}$. The scattering geometry is sketched in inset of Figure 1 in the main manuscript. As expected the maximum in the RRS signal and the emission spectra peak overlap very nicely.

It is apparent in Figure S6 that both absolute RRS intensity as well as resonant enhancement in (H,V) geometry constitutes 5800% from the non-resonant Rayleigh scattering intensity and is significantly lower in (V,V) with 900%. This is very striking due to the fact that the non-resonant Rayleigh scattering signal is normally much larger in (V,V) compared to (H,V)-geometry due to spurious signal by scattering on imperfection on sample surface or by scattering on imperfections on windows and other optical elements in the optical path that is always co-polarized. The polarization dependence of the RRS signal follows the

identical polarization selection rules found in RILS spectra for ν=2+2/5 shown in Figure 5 of the main text. The observation that RRS and RILS signal exhibit the same anisotropy concerning the scattering geometry support the interpretation that such a polarization dependence is caused by an anisotropy in the susceptibility $\chi$ parallel and perpendicular to the in-plane component of the magnetic field $\chi_{//}$ and $\chi_{\perp}$, respectively.

Similar to observation in RILS signal shown in the main text also the RRS signal feature a striking dependence on filling factor. By tuning the filling factor slightly away from ν=2+2/5 by δν=0.02 the absolute value as well as the resonant enhancement of the RRS signal is greatly reduced by one order of magnitude for both polarization direction. In (H,V) geometry the enhancement is reduced to 440% and in (V,V) to 100%. This striking filling factor dependence of both magnitude and polarization dependence is in agreement with the interpretation introduced in the main manuscript as a hint for the existence of nematic FQHE states at 2+2/5, an incompressible quantum fluid without rotational symmetry.

We would like to mention that the non-resonant Rayleigh scattering signal in (V,V) geometry is larger by a factor of 2 to 4 for ν=2.38 compared to ν=2+2/5. The magnitude of the non-resonant Rayleigh signal in (H,V) geometry is similar for both filling factors. This difference in the non-resonant behavior can be explained by a larger impact of spurious elastic (Rayleigh) scattering that is co-polarized at ν=2.38. This is also the origin of the larger intensity at the tail of the $E$=0meV mode in (V,V) geometry taken at ν=2.38 visible at the RILS spectra (blue traces) in Figure 5 (b) of the main manuscript compared to the RILS measurements taken at ν=2+2/5 (Figure 5(a)). The origin of another rather broad increase in the Rayleigh scattering signal in (V,V) geometry at ν=2.38 for energies larger that the N=1LL emission energies is unclear. This additional RRS signal might be related to another emission line. A hint for another higher energy emission line is seen as shoulder in the emission line at similar energies. Its origin is unclear and we can only speculate that it might be due to emission from a conduction band state with another close-by valence band state or emission stemming for a localized impurity in agreement that in RRS only (V,V) geometry is sensitive at the specific energy.

**References**


[1] A. Pinczuk, B. S. Dennis, L. N. Pfeiffer, and K. W. West, Phys. Rev. Lett. **70**, 3983 (1993).

[2] B. B. Goldberg, D. Heiman, M. J. Graf, D. A. Broido, A. Pinczuk, C. W. Tu, J. H. English, and A. C. Gossard, Phys. Rev. B **38(14)** 10131 (1988).

[3] C. F. Hirjibehedin, I. Dujovne, I. Bar-Joseph, A. Pinczuk, B. S. Dennis, L. N. Pfeiffer, and K. W. West, Solid State Commun. **127**, 799 (2003).
